# Supplementary material for: SoK: An Introspective Analysis of RPKI Security
Source: arXiv:2408.12359 source file (2024-08-22)
Supplement: Supplementary file 1 [file appendix.tex]

Figure \ref{fig:roa-trend} depicts the graph of ROAs and VRPs for all RIRs during our observation periods. Figure \ref{fig:roa-trend-1} and \ref{fig:roa-trend-2} show the number of ROAs (first column) and VRPs (second column) observed during every validation iteration for R1 and R2 respectively. The first thing we notice is gradual increase of both ROAs and VRPs across all RIRs. This is in line with the gradual but steady adoption of RPKI worldwide. Additionally, we also notice occasional blackouts that lead to VRPs disappearing from RP view, which in turn means routers will also lose access to those VRPs therefore downgrading protection. An outage is most dangerous when it lasts for multiple hours or days. An outage of this length can lead to router caches being flushed of the missing ROAs. It is important to note that the ROA column shows the number of the validated ROA files, and one ROA file can contain multiple VRPs. A drop in the number of processed ROA does not necessarily correlate to loss of VRPs. ROA files can carry multiple VRPs, thus operators can aggregate existing ROAs into one, or add new VRPs to existing ROAs without increasing the number of ROAs served. By this token, a drop in the number of ROAs that is not accompanied by loss of VRPs does not necessarily signal an issue but active operator refactoring. If a sharp drop in ROAs is followed by small drop in VRPs, it implies those ROAs carried very few VRPs in them. We classify ROA and VRP graph anomalies in three scenarios: 1) ROA graph drops corresponds to actual VRP loss and is immediately visible 2) ROA loss raises alarms but the VRP loss is limited 3) invisible ROA anomaly on graph but tangible loss of VRPs.

\indent \textbf{RIPE} RIR is one of the steadiest RIRs. Figure \ref{fig:roa-trend-1} shows a contiguous increase in ROAs and VRPs, as is expected, given the increasing global adoption of RPKI and no large outages. Figure \ref{fig:roa-trend-2} shows 3 small outages ($\sim$ 2023-08-15, $\sim$2023-08-29/30 and $\sim$2023-10-27) as detected on the ROA graph. The first outage is an example of (1), and led to the loss of approximately 110 ROA files and 505 contained VRPs. This outage can be proportionally seen in both ROA and VRP graphs and it lasted for a total of 18 hours. The second failure is an instance of (2), which lasted for over 48h and affected on average 130 ROA files and 168 VRPs. This second outage is mostly visible in the ROA graph but not so much on the VRP graph, mostly due to ROAs containing 1.2 VRPs on average, a very low number. The last type of outage is a demonstration of scenario (3). We don't notice anything on the ROA graph but the VRP plot shows us loss of ROAs that lasted for multiple days. Due to RIPE having many clients that use the delegated RPKI, the outages did not happen as a result of one repository failing, but multiple repositories under RIPE. The failures range from manifest and certificate expirations, to DNS query failures.\\
\indent In November 2022, we noticed \textbf{AFRINIC} RIR experience a blackout of over 4,000 VRPs which lasted almost 7h, from 01:09:50 - 08:22:47. The root cause of the issue according to the logs was the manifest file not being correctly validated. Because AFRINIC does not offer delegated RPKI operations and all resources are centrally managed, one internal uncaught misconfiguration can affect multiple resource holders. In September 5th-6th 2023 a similar error occurred, this time because of prematurely issued and expired certificates with the error codes: \textit{"certificate is not yet valid"} and \textit{"certificate has expired"}. Over a period of 2 days over 200 VRPs were not being correctly propagated.\\
\indent The \textbf{APNIC} tree consists of a set of sturdy PPs. We observe in R1 no meaningful errors. In R2 we notice one single outlier outage that lasts for a handful of validation intervals due to errors in the Amazon PP certificate and manifest file. This outage did not last long enough to cause longterm ROA propagation damage. Missing a handful of validation rounds does not necessarily translate to outage as the error was caught in less than an hour. \\
\indent Similarly, \textbf{LACNIC} suffered 3 large-scale outages on September 8th, December 17th and January 31st in R1, due to internal configuration issues that led to invalid notifications. According to Figure \ref{fig:roa-trend-2} the number of announced VRPs dropped by over a 1,000 in late October and is still not back up. Since this does not seem to be a temporary outage, it suggests either an ongoing issue with the resource owner, some VRPs were removed from the internet completely or those prefixes migrated under the umbrella of another RIR. Just like AFRINIC, LACNIC has a very centralized approach to RPKI and so far has only allowed one child PP.\\
\indent The \textbf{ARIN} repository showed considerable volatility in 2022, see Figure \ref{fig:roa-trend-1}. A few repositories under this TAL were occasionally affected by processing errors due to expired certificates and for a month's period over 10,000 ROAs would often vanish from the ecosystem in odd blackouts. That massive oscillation of VRP content in the cache can affect the router RPKI cache as well. Due to the periodic nature of the blackout, such a situation might lead to short-lived deletion of ROA statuses from BGP caches. According to our followup measurements later in the year during R2, see Figure \ref{fig:roa-trend-2}, ARIN stability has improved considerably and is now one of the most stable RIRs, rivaling RIPE.

\begin{figure}
    \centering
    \begin{subfigure}{0.49\textwidth}
        \includegraphics[width=\linewidth]{figs/day_errors_round1.png}
        \caption{September 22 - February 23}
        \label{fig:day-round-1}
    \end{subfigure}
    \begin{subfigure}{0.49\textwidth}
        \includegraphics[width=\linewidth]{figs/day_errors_round2.png}
        \caption{August - September 2023}
        \label{fig:day-round-2}
    \end{subfigure}
    \caption{Total daily errors}
    \label{fig:day-errors}
\end{figure}

\begin{figure*}
    \centering
    \begin{subfigure}{0.25\textwidth}
        \includegraphics[width=\linewidth]{figs/to_legend.png}
        \vspace{0.5pt}
        \caption{TimeOut Error Legend}
        \label{fig:to-legend}
    \end{subfigure}
    \begin{subfigure}{0.30\textwidth}
        \includegraphics[width=\linewidth]{figs/to_daily_errors_round1.png}
        \caption{R1: TimeOut day errors}
        \label{fig:day-to-errors-1}
    \end{subfigure}
        \begin{subfigure}{0.30\textwidth}
        \includegraphics[width=\linewidth]{figs/to_daily_errors_round2.png}
        \caption{R2: TimeOut day errors}
        \label{fig:day-to-errors-2}
    \end{subfigure}
        \begin{subfigure}{0.30\textwidth}
        \includegraphics[width=\linewidth]{figs/nto_legend.png}
        \vspace{0.5pt}
        \caption{Non-TimeOut Error Legend}
        \label{fig:nto-legend}
    \end{subfigure}
    \begin{subfigure}{0.30\textwidth}
        \includegraphics[width=\linewidth]{figs/nto_daily_errors_round1.png}
        \caption{R1: Non-TimeOut day errors}
        \label{fig:day-nto-errors-1}
    \end{subfigure}
    \begin{subfigure}{0.30\textwidth}
        \includegraphics[width=\linewidth]{figs/nto_daily_errors_round2.png}
        \caption{R2: Non-TimeOut day errors}
        \label{fig:day-nto-errors-2}
    \end{subfigure}
    \caption{Breakdown of most common errors daily}
    \label{fig:day-error-rates}
\end{figure*}

\begin{figure}
    \centering
    \begin{subfigure}{0.49\textwidth}
            \includegraphics[width=\linewidth]{figs/mon-rrdp-A.png}
    \caption{RRDP-Triggered A Requests per Validation Interval}
    \label{fig:mon-rrdp-a}
    \end{subfigure}
    \begin{subfigure}{0.49\textwidth}
    \includegraphics[width=\linewidth]{figs/mon-rrdp-aaaa.png}
    \caption{RRDP-Triggered AAAA Requests per Validation Interval}
    \label{fig:mon-rrdp-aaaa}
    \end{subfigure}
    \caption{RRDP Requests}
    \label{fig:mon-rrdp}
\end{figure}
\indent Figure \ref{fig:mon-rrdp-a} and \ref{fig:mon-rrdp-aaaa} show the number of A and AAAA requests sent for every query. The numbers for both categories match, which means for every HTTP request the resolver will send both A and AAAA simultaneously. The number of A/AAAA requests is higher than contacted RRDPs in Figure \ref{fig:mon-rrdp} due to retries. Not all retries are visible in the logs but are triggered by the RP software itself as redundancy.
%Additionally, not all failures lead to rsync fallback requests, the internal stub resolver sends additional requests sometimes to resolve the issue with RRDP. We notice that for every validation interval, the RP sends DNS requests from scratch. It is possible the stub resolver on our machine does not store the domain/IP data in a cache and for every interval a new query is necessary. 
On average the number of DNS requests for every validation interval is 132, 66 A and 66 AAAA requests per interval. That's almost double traffic requests proportionally to the amount of PPs to be queried.\\

\begin{figure}
    \centering
    \begin{subfigure}{0.50\textwidth}
    \includegraphics[width=\linewidth]{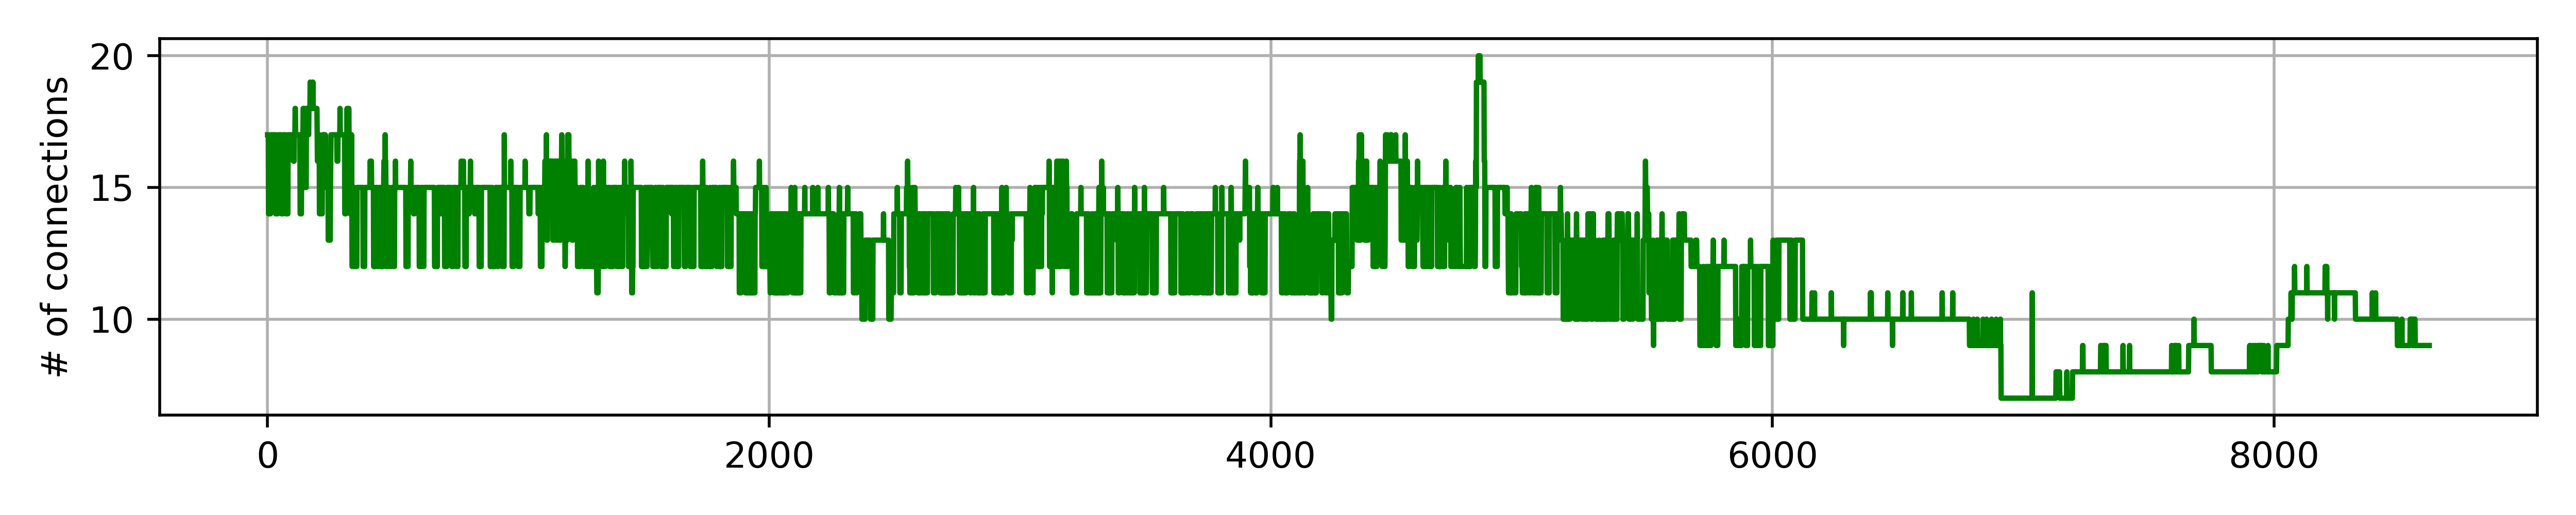}
    \caption{Rsync-Triggered A Requests per Validation Interval}
    \label{fig:mon-rsync-a-appendix}
    \end{subfigure}
    \begin{subfigure}{0.50\textwidth}
    \includegraphics[width=\linewidth]{figs/mon-rsync-aaaa.png}
    \caption{Rsync-Triggered AAAA Requests per Validation Interval}
    \label{fig:mon-rsync-aaaa}
    \end{subfigure}
    \caption{Rsync Requests}
    \label{fig:mon-rsync-appendix}
\end{figure}
\vspace{-20pt}
\indent Figure \ref{fig:mon-rsync-a} and \ref{fig:mon-rsync-aaaa} shows the number of A and AAAA record requests per validation cycle triggered by rsync. If we compare the absolute number of requests with the number of unique rsync requests in Figure \ref{fig:mon-rsync}, the RP sends more DNS requests than the number of PPs it needs to query. This is due to errors in the repository connection, failures against the initial query incentivizes retries. This is the same behavior we observed for RRDP. If we look however at the average number of A/AAAA queries it is slightly higher than 12. This means that while there are retries as visible from the graph, they do not happen as often as with RRDP and the average of rsync requests with the A/AAAA queries send match up. \\

\indent Figure \ref{fig:mon-duration} shows the average processing time of our RP, with a global average of 178 seconds before the november anomaly and a mere 66 seconds during. We see in the graph that in early november, the average processing time decreased considerably for 15 days. Further, Figure \ref{fig:mon-wait} shows the average wait time between validation intervals. While the default Routinator interval is 600 seconds (10 minutes), we observe that the average waiting time is 556 seconds with a standard deviation of 231 seconds (3.85 minutes). This is an internal anomaly of the relying party which is not specified in the source code per se, so this is not an attempt at query randomization. Routinator, despite being the most widely used RP on the internet, does not necessarily respect its own waiting intervals and exhibits even major delays in validation, that range from 1000 to 2000 seconds.\\
\begin{figure}
\centering
    \includegraphics[width=\linewidth]{figs/mon-duration.png}
    \caption{Duration of Validation Intervals}
    \label{fig:mon-duration}
\end{figure}
\begin{figure}
    \centering
    \includegraphics[width=\linewidth]{figs/mon-btw-intervals.png}
    \caption{Wait time between validation intervals}
    \label{fig:mon-wait}
\end{figure}
\indent \textit{The November Performance Improvement.} The takeaway from Figures \ref{fig:mon-rrdp-pp} - \ref{fig:mon-duration} is that the RPKI network is quite volatile, with chronic delaying errors being the norm and periods of good networking conditions appearing as graph anomalies. We correlate this data with Figure \ref{fig:dns-res} and observe that good network hygiene leads to a dramatic increase in processing speed, namely validation processes became about 2.6x faster.  These numbers show that RPKI health is heavily dependent on the health of PPs themselves, their availability, connectivity, bandwidth and responsible deployment.
